# Supplementary material for: The Teaching Dimension of Kernel Perceptron
Source: arXiv:2010.14043 source file (2021-02-24)
Supplement: Supplementary file 1 [file appendix_theory_linear.tex]

\section{Linear Perceptrons}\label{appendix: linear perceptron}
